# Supplementary material for: WeditGAN: Few-Shot Image Generation via Latent Space Relocation
Source: arXiv:2305.06671 source file (2024-01-14)
Supplement: Supplementary file 1 [file version2.tex]

\section{Version Updates}
\label{sec:version}

Compared with the previous version (v1), this version mainly updates the following contents.
\begin{itemize}
    \item Recompute the quantitative results of all the experiments following the evaluation settings of previous works, so that these results can now be directly and fairly compared with those reported in previous works. See \textbf{Evaluation Method} in \cref{sec:supp_detail}.
    \item Add the latest method RICK \cite{rick} to the baseline list. Remove the earliest one EWC \cite{ewc}.
    \item Other modifications.
\end{itemize}
